# Supplementary material for: Frontier Orbitals and Quasiparticle Energy Levels in Ionic Liquids
Source: arXiv:2006.16717 ancillary file (2020-06-30)
Supplement: Supplementary file 1 [file Supplementary_information_v1.pdf]

# Supplementary Information

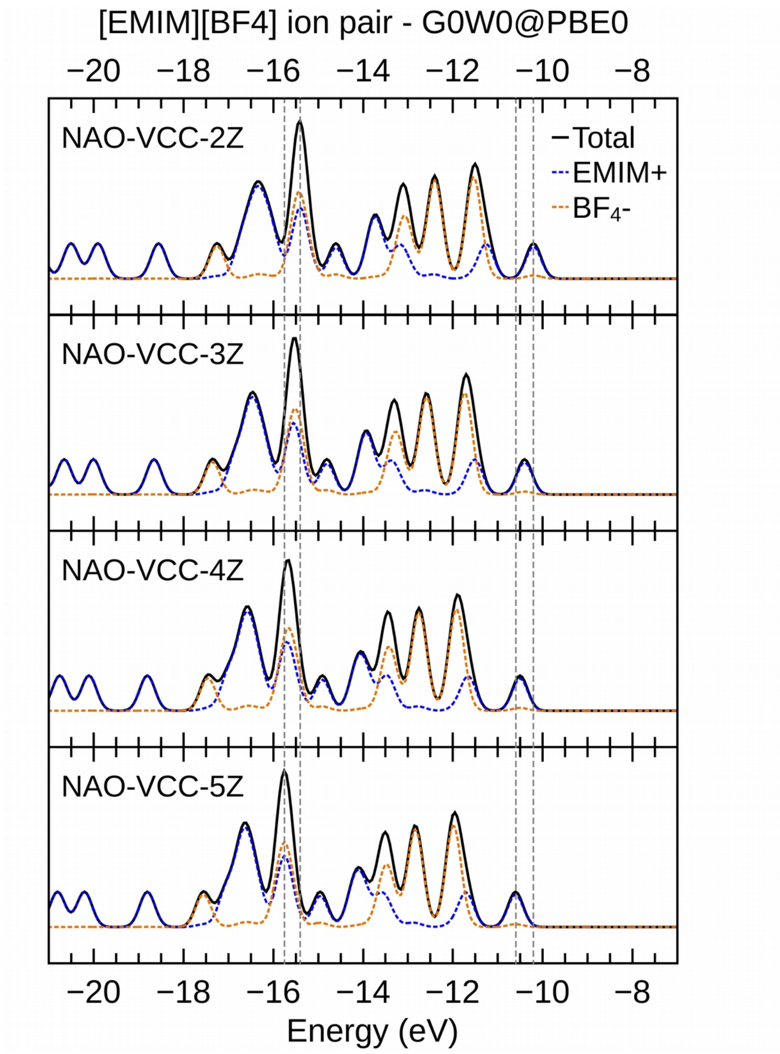


Supplementary Figure 1: basis set convergence in G0W0 calculations of the [EMIM][BF4] ion pair.

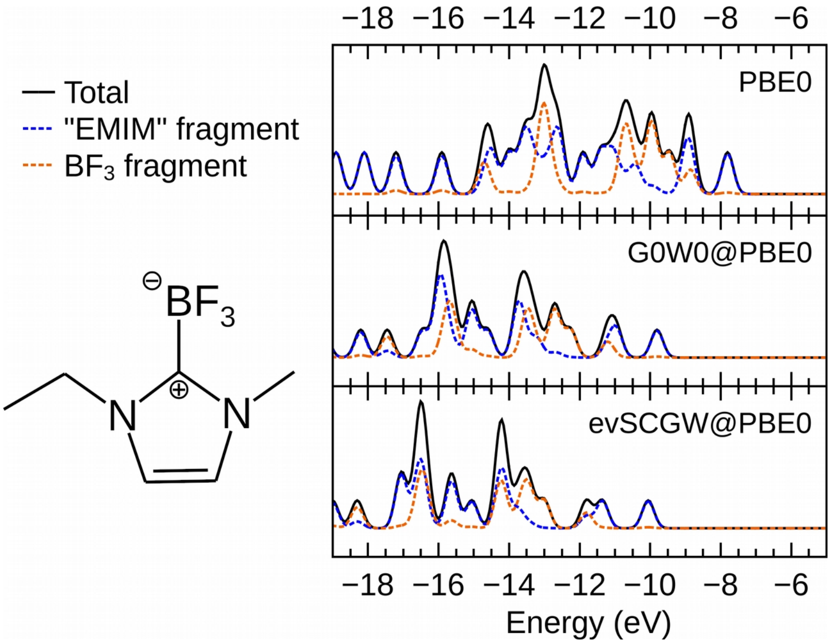


Supplementary Figure 2: the density of states of the EMIM-BF3 adduct from different levels of theory.

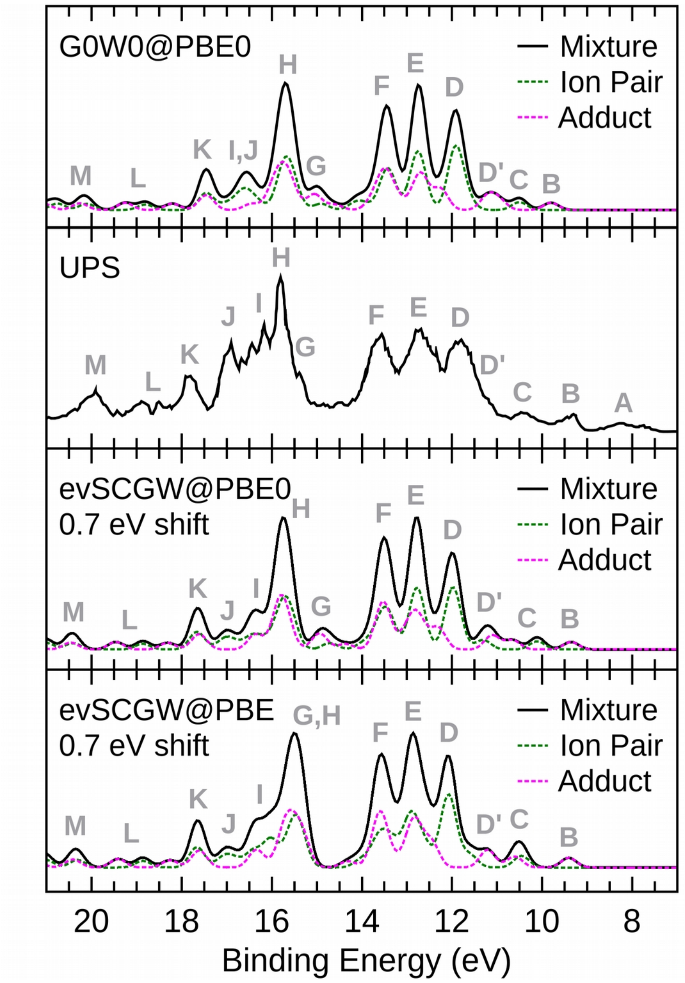


Supplementary Figure 3: simulated spectra of the [EMIM][BF4] ion pair and the adduct from different levels of theory.

# The structures used in the GW calculations

All atomic positions are given in Angstroms. The .xyz format is used for molecules, and the XcrysDen .xsf format is used for crystals.

### [EMIM][BF4] ion pair

```
24
Atoms
F    2.5240652  7.63637794 8.48746933
F    2.74309965 9.89425493 8.86046196
B    3.17688035 8.65335119 9.22843914
C    4.14603599 5.05371791 7.73075575
H    3.31314301 5.75162748 7.68335536
H    4.81627053 5.24922076 6.89721619
F    2.91669847 8.40015274 10.59845826
F    4.56499651 8.50737136 9.02520144
H    3.79513102 4.02361324 7.68975606
N    4.86109364 5.29341179 8.97143036
C    4.36107503 5.93970912 10.01450083
C    6.16862612 4.9768014  9.23908596
H    3.37397131 6.36817306 10.07431746
N    5.29956917 6.04512452 10.9426412
H    6.78647729 4.45200449 8.5334801
C    6.4450285  5.45194566 10.47566448
C    5.16167091 6.82477283 12.17269149
H    7.35253487 5.42328265 11.05031863
H    4.10342617 7.05785674 12.26672812
C    5.97291417 8.10234745 12.11639021
H    5.45700137 6.18380434 13.00467302
H    5.66403021 8.70193084 11.26174407
H    5.79809563 8.67564059 13.02642239
H    7.04298687 7.90138797 12.04591018
```

**EMIM-BF3 adduct**

```
22
Atoms
C     3.44091089 4.54708165 8.25997677
H     2.43296589 4.72518877 8.62222525
H     3.54485516 4.943866   7.25265039
H     3.63611457 3.47593563 8.25928579
N     4.38154763 5.22871825 9.12973004
C     4.20790636 5.40820682 10.44706184
C     5.58944256 5.73883286 8.73052953
B     2.85027156 4.90807095 11.27886722
N     5.31159333 6.03405708 10.87879749
H     5.92727671 5.69324587 7.71103214
C     6.17431956 6.25290667 9.83367799
C     5.55597654 6.50003619 12.24130684
H     7.1192792  6.74881422 9.96314816
H     5.12723221 5.76781415 12.91880047
C     4.9607292  7.87087648 12.48952395
H     6.63781135 6.50538712 12.37718502
H     3.87703101 7.83827455 12.38505146
H     5.19337213 8.19300448 13.50471533
H     5.36110663 8.6119306  11.79592923
F     2.74244287 3.53877205 11.07712452
F     1.76898364 5.58159117 10.71805225
F     2.99175451 5.2163003  12.62252238
```

**[EMIM][OTf] ion pair**

```
27
Atoms
N     7.97762469 8.12799022 0.41293065
C     6.89235661 8.65333701 0.97168391
H     5.95347642 8.81387033 0.47917125
N     7.12831206 8.86391169 2.26315218
C     8.40575397 8.44046968 2.54438802
H     5.71453861 8.36613244 3.70720625
C     8.06646163 7.6487284  -0.97781595
C     8.93861545 7.98358959 1.38581784
C     6.12783431 9.26024733 3.25047074
H     8.81207158 8.48441933 3.53569334
C     8.50873124 6.19555055 -1.04363302
H     8.75214972 8.30540989 -1.51205679
H     7.07168359 7.75354934 -1.39871285
H     9.89918426 7.55554164 1.18144092
H     5.32582422 9.79126181 2.75049585
H     6.59789606 9.90496821 3.98744011
H     9.52762718 6.06619695 -0.68086518
H     8.48213194 5.86973295 -2.08192307
H     7.83569225 5.57292639 -0.46186737
C     4.23725334 4.5098194  1.3842376
S     5.21712946 6.08955034 1.2435108
F     4.08154426 4.15779914 2.66845855
F     3.02092798 4.64795368 0.84068536
F     4.86305363 3.50519972 0.7522115
O     5.30068187 6.32382971 -0.19090439
O     6.4900869  5.77325825 1.87163909
O     4.41972875 7.06941201 1.96339068
```

**[EMMIM][NTf2] ion pair**

```
37
Atoms
N     1.68890358 3.21739333 -0.31650913
C     3.61929938 1.62071854 -0.21604167
H     4.23692496 2.51071556 -0.13926168
H     3.88301914 1.10441149 -1.14194479
H     3.84309414 0.97464692 0.63350819
C     2.19216995 1.98420203 -0.23553222
N     1.16357205 1.13615531 -0.17228728
C     -0.00979415 1.84638106 -0.22494352
H     -0.96955627 1.36395344 -0.2229604
C     0.32105168 3.14946185 -0.31909956
H     -0.28939415 4.02392171 -0.43978078
C     2.45693989 4.43378159 -0.50111987
H     3.0126046  4.67631034 0.4036631
H     1.76369126 5.2340674  -0.73646751
H     3.13024047 4.3131405  -1.34564042
C     1.24539182 -0.31995345 -0.17777238
H     0.49022611 -0.68138212 0.52087564
H     2.21734055 -0.59594344 0.22734017
C     1.04873986 -0.89839906 -1.56485918
H     0.07912842 -0.61652732 -1.97483304
H     1.09287012 -1.98626781 -1.5113755
H     1.82383706 -0.55024041 -2.2456728
N     2.05827813 2.53449582 -3.37162791
S     1.00865834 3.51222144 -4.04486435
O     1.36579836 4.05122097 -5.31332995
O     0.52443094 4.3933401  -3.02153952
C     -0.43907777 2.40203586 -4.38292096
F     -0.13158245 1.45400164 -5.25066468
F     -1.44015333 3.12368463 -4.86904001
F     -0.86135295 1.81417746 -3.25771493
S     3.17720687 1.7161485  -4.13050892
O     2.94712369 1.42776501 -5.50492319
O     3.59479466 0.65407169 -3.25624741
C     4.63085057 2.8687278  -4.10550914
F     4.39835312 3.96735197 -4.79993247
F     5.69296357 2.25583722 -4.60704225
F     4.91790784 3.22807251 -2.84451968
```

**[BMIM][PF6] crystal** – experimental structure from Choudhury et al., JACS 127, 16792 (2005)

```
CRYSTAL

PRIMVEC
        8.7740001678          0.0000000000          0.0000000000
       -2.0134835928          8.7144147359          0.0000000000
       -3.8070843567         -1.8404016396          7.9809803322

CONVVEC
        8.7740001678          0.0000000000          0.0000000000
       -2.0134835928          8.7144147359          0.0000000000
       -3.8070843567         -1.8404016396          7.9809803322

PRIMCOORD
64 1
P     3.707303286         1.737852931         3.583939075
P    -0.753871202         5.136159897         4.397041798
F     2.699795008         1.367598653         4.743256092
F     0.253637135         5.506414413         3.237724066
F     2.984874010         0.720257699         2.583682775
F    -0.031441726         6.153755188         5.397297859
F     4.726287842         2.143983841         2.416800499
F    -1.772855639         4.730029106         5.564180374
F     4.709149361         0.589570820         4.054737091
F    -1.755717516         6.284442425         3.926243067
F     4.447157383         2.772157907         4.557458878
F    -1.493725300         4.101855278         3.423521519
F     2.729165077         2.894247532         3.095343351
F     0.224267572         3.979765415         4.885636806
N    -1.545015335         1.293593645         7.129808903
N     4.498447895         5.580419064         0.851171494
N    -0.724282444         0.803206444         5.193543434
N     3.677715063         6.070806503         2.787436962
C    -1.615914822         1.553129554         5.830106258
C     4.569347382         5.320883751         2.150874376
C    -0.053381436         0.039914027         6.119018078
C     3.006813765         6.834099293         1.861962438
C    -0.573873460         0.337348849         7.323347569
C     3.527305841         6.536664009         0.657632947
C     1.378056288         3.694595575         0.182764336
C     1.575376391         3.179417133         7.798215866
C     0.348462820         2.676091671         0.650450349
C     2.604969263         4.197921276         7.330530167
C     4.397556305         0.351273298         7.538834095
C    -1.444123864         6.522739887         0.442146420
```

| | | | |
|---|---|---|---|
| C | 7.152211189 | 1.209235191 | 0.069434635 |
| C | -4.198779106 | 5.664778233 | 7.911545753 |
| C | -0.484963566 | 0.823778272 | 3.743877888 |
| C | 3.438395977 | 6.050234795 | 4.237102509 |
| H | -2.219220400 | 2.176003456 | 5.419085979 |
| H | 5.172653198 | 4.698009014 | 2.561894655 |
| H | 0.669882655 | -0.568317592 | 5.945032120 |
| H | 2.283550024 | 7.442329884 | 2.035948277 |
| H | 3.471698523 | 1.776049852 | 0.181167871 |
| H | -0.518266082 | 5.097963333 | 7.799812317 |
| H | -2.866805315 | 2.642857313 | 7.834928513 |
| H | 5.820237637 | 4.231155396 | 0.146051913 |
| H | 1.918235540 | 3.943326712 | 0.936967492 |
| H | 1.035196543 | 2.930686235 | 7.044013023 |
| H | -0.192402035 | 3.056958199 | 1.345592976 |
| H | 3.145834208 | 3.817055225 | 6.635387421 |
| H | 0.802533031 | 1.915330172 | 1.020767450 |
| H | 2.150899172 | 4.958682537 | 6.960213184 |
| H | 4.925357819 | -0.081435829 | 6.864440918 |
| H | -1.971924901 | 6.955449104 | 1.116539359 |
| H | 3.969005823 | 1.110866189 | 7.135794640 |
| H | -1.015573144 | 5.763146400 | 0.845185757 |
| H | 7.576690674 | 0.441442132 | 0.458906412 |
| H | -4.623258114 | 6.432570934 | 7.522074223 |
| H | 2.793550968 | -0.908714890 | 7.315366745 |
| H | 0.159881502 | 7.782728195 | 0.665613830 |
| H | 6.609444618 | 1.644889116 | 0.731057346 |
| H | -3.656012297 | 5.229123592 | 7.249923229 |
| H | -1.233505011 | 1.237798929 | 3.308914661 |
| H | 4.186937332 | 5.636213779 | 4.672065735 |
| H | -0.391502976 | -0.077981442 | 3.429427147 |
| H | 3.344935656 | 6.951994419 | 4.551552773 |
| H | 0.313547760 | 1.317525268 | 3.545151472 |
| H | 2.639884472 | 5.556487560 | 4.435828686 |

**[BMIM]Cl crystal** – experimental structure from Holbrey et al., Chem. Commun. 14, 1636 (2003)

```
CRYSTAL

PRIMVEC
      10.1129999161    0.0   0.0
      0.0   11.4110002518    0.0
      0.0   0.0   8.328499794

CONVVEC
      10.1129999161    0.0   0.0
      0.0   11.4110002518    0.0
      0.0   0.0   8.328499794

PRIMCOORD
104 1
Cl    0.597476065      6.556418419      3.422513723
Cl    9.515523911      4.854581833      7.586763382
Cl    5.653975964      10.560082436     3.422513723
Cl    4.459023952      0.850917637      7.586763382
N     2.697137117      3.013644934      2.352801085
N     7.41586256       8.397356033      6.51705122
N     7.753637314      2.691855192      2.352801085
N     2.359362841      8.719144821      6.51705122
N     2.495888472      2.811670542      4.484897137
N     7.617111683      8.599329948      0.320647836
N     7.552388191      2.893829584      4.484897137
N     2.560611486      8.517170906      0.320647836
C     2.094402313      3.512305737      3.418848991
C     8.018597603      7.898694515      7.583098888
C     7.150902748      2.193194389      3.418848991
C     2.962097645      9.217805862      7.583098888
C     3.398979425      1.837171078      4.065140724
C     6.714020729      9.573828697      8.229390144
C     8.455478668      3.868329048      4.065140724
C     1.657520533      7.542671204      8.229390144
C     3.514267445      1.983231902      2.732580662
C     6.598732948      9.427768707      6.896830559
C     8.570767403      3.722268343      2.732580662
C     1.542232513      7.68873167       6.896830559
C     2.032712936      3.039890528      5.861598492
C     8.08028698       8.371109962      1.697347999
C     7.089212894      2.665609598      5.861598492
C     3.023787022      8.745389938      1.697347999
C     2.57679224       3.570502043      0.981097281
C     7.536208153      7.840497971      5.145347118
```

| | | | |
|---|---|---|---|
| C | 7.633291721 | 2.134998083 | 0.981097281 |
| C | 2.479707718 | 9.27600193 | 5.145347118 |
| C | 3.458646059 | 4.788055897 | 0.797870278 |
| C | 6.654354095 | 6.622944355 | 4.962120056 |
| C | 8.515146255 | 0.917444289 | 0.797870278 |
| C | 1.597853899 | 10.493556023 | 4.962120056 |
| C | 4.960426331 | 4.47881794 | 0.823688626 |
| C | 5.152573586 | 6.932182312 | 4.987938881 |
| C | 10.016925812 | 1.226682425 | 0.823688626 |
| C | 0.096073471 | 10.184318542 | 4.987938881 |
| C | 5.80789566 | 5.715769768 | 0.634631693 |
| C | 4.305104256 | 5.695230484 | 4.798881531 |
| C | 0.751396418 | 11.400731087 | 0.634631693 |
| C | 9.361603737 | 0.010270244 | 4.798881531 |
| H | 1.537175894 | 4.165015221 | 3.48131299 |
| H | 8.575823784 | 7.245985031 | 7.645562649 |
| H | 6.59367609 | 1.540484905 | 3.48131299 |
| H | 3.519323826 | 9.87051487 | 7.645562649 |
| H | 3.832827091 | 1.312265038 | 4.647303104 |
| H | 6.280172825 | 10.098734856 | 0.483053714 |
| H | 8.889327049 | 4.393235207 | 4.647303104 |
| H | 1.223672867 | 7.017765045 | 0.483053714 |
| H | 3.974409103 | 1.529074073 | 2.14042449 |
| H | 6.138590813 | 9.881926537 | 6.304674149 |
| H | 9.030908585 | 4.176425934 | 2.14042449 |
| H | 1.082090974 | 7.234574318 | 6.304674149 |
| H | 1.436046004 | 2.476186991 | 6.104790211 |
| H | 8.676953316 | 8.934813499 | 1.940540791 |
| H | 6.492546082 | 3.229312897 | 6.104790211 |
| H | 3.620453835 | 8.181687355 | 1.940540791 |
| H | 1.486611009 | 3.822685242 | 5.854935646 |
| H | 8.62638855 | 7.588314533 | 1.690685987 |
| H | 6.543111324 | 1.882815003 | 5.854935646 |
| H | 3.56988883 | 9.528185844 | 1.690685987 |
| H | 2.497910976 | 2.761461973 | 6.537872791 |
| H | 7.61508894 | 8.64953804 | 2.373623133 |
| H | 7.554410934 | 2.944038153 | 6.537872791 |
| H | 2.55858922 | 8.466961861 | 2.373623133 |
| H | 2.841752768 | 2.852750063 | 0.491381496 |
| H | 7.27124691 | 8.558250427 | 4.655631542 |
| H | 7.898252964 | 2.852750063 | 0.491381496 |
| H | 2.21474719 | 8.558250427 | 4.655631542 |
| H | 1.790001035 | 3.822685242 | 0.866163969 |
| H | 8.322999001 | 7.588314533 | 5.030413628 |
| H | 6.846500874 | 1.882815003 | 0.866163969 |
| H | 3.266499043 | 9.528185844 | 5.030413628 |

| | | | |
|---|---|---|---|
| H | 3.256386042 | 5.45445776 | 1.565757871 |
| H | 6.856613636 | 5.956542492 | 5.730007648 |
| H | 8.312886238 | 0.251042187 | 1.565757871 |
| H | 1.800114036 | 11.159957886 | 5.730007648 |
| H | 3.205821037 | 5.180593967 | 8.245214462 |
| H | 6.907178402 | 6.230406284 | 4.080965042 |
| H | 8.262321472 | 0.524906039 | 8.245214462 |
| H | 1.850678921 | 10.886094093 | 4.080965042 |
| H | 5.208194733 | 4.005261421 | 1.699013948 |
| H | 4.904805183 | 7.405738831 | 5.863263607 |
| H | 0.151694849 | 1.700238943 | 1.699013948 |
| H | 9.961304665 | 9.71076107 | 5.863263607 |
| H | 5.147517204 | 3.78845191 | 0.083284996 |
| H | 4.965482712 | 7.622548103 | 4.247534752 |
| H | 0.091017634 | 1.917048216 | 0.083284996 |
| H | 10.021983147 | 9.493952751 | 4.247534752 |
| H | 5.653167248 | 6.401570797 | 1.390859485 |
| H | 4.459832668 | 5.009429455 | 5.555109501 |
| H | 0.596667171 | 10.714929581 | 1.390859485 |
| H | 9.516332626 | 0.69607091 | 5.555109501 |
| H | 6.694806099 | 5.317525864 | 0.424753487 |
| H | 3.418194056 | 6.093474388 | 4.589003563 |
| H | 1.638305426 | 0.387974113 | 0.424753487 |
| H | 8.474694252 | 11.023025513 | 4.589003563 |
| H | 5.521697998 | 6.150528908 | 8.111958504 |
| H | 4.591301918 | 5.260471344 | 3.947708845 |
| H | 0.46519804 | 10.965971947 | 8.111958504 |
| H | 9.647802353 | 0.445029408 | 3.947708845 |

**[EMIM][BF4] crystal** – experimental structure from Choudhury et al., JACS 127, 16792 (2005)

```
CRYSTAL

PRIMVEC
        8.7617998123          0.0000000000          0.0000000000
        0.0000000000          9.3961000443          0.0000000000
       -1.7320365008          0.0000000000         11.2925429672

CONVVEC
        8.7617998123          0.0000000000          0.0000000000
        0.0000000000          9.3961000443          0.0000000000
       -1.7320365008          0.0000000000         11.2925429672

PRIMCOORD
96 1
B      6.970133781          7.059477806          6.211575985
B      0.059629574          2.336622000          5.080967426
B      3.574511290          2.361428022         10.727238655
B      3.455251932          7.034672260          0.565305114
F      6.044565678          6.998027325          5.175711632
F      0.985197902          2.398072720          6.116831779
F      6.232115746          2.299978018          0.470560223
F      0.797647178          7.096122742         10.821983337
F      6.504496098          7.913583279          7.185219288
F      0.525267065          1.482516527          4.107324123
F      4.040148735          3.215533972          9.753595352
F      2.989614487          6.180566788          1.538948536
F     -0.564502656          7.483805656          5.726674557
F      7.594265938          1.912294269          5.565868855
F      2.347347975          2.785755157         11.212140083
F      4.682415485          6.610344410          0.080403060
F      7.115749359          5.777474403          6.753731728
F     -0.085985817          3.618625879          4.538811684
F      3.428896189          1.079424739         10.185083389
F      3.600867987          8.316676140          1.107460022
N      7.761333942          7.954268456          0.423583299
N     -0.731570661          1.441831708         10.868960381
N      4.515347481          3.256218433          5.222688198
N      2.514415264          6.139881611          6.069854736
N      6.927999020          8.836468697          2.205320835
N      0.101764463          0.559631705          9.087223053
N      5.348682880          4.138417721          3.440950871
N      1.681080222          5.257681847          7.851592064
C      6.752040386          8.667714119          0.908146381
C      0.277722895          0.728385806         10.384396553
```

| | | | |
|---|---|---|---|
| C | 5.524641037 | 3.969664335 | 4.738125324 |
| C | 1.505122185 | 5.426435947 | 6.554418087 |
| C | 8.099196434 | 8.204956055 | 2.580007315 |
| C | -1.069433689 | 1.191143751 | 8.712536812 |
| C | 4.177484512 | 3.506906271 | 3.066264391 |
| C | 2.852278948 | 5.889194012 | 8.226278305 |
| C | -0.143302515 | 7.652559757 | 1.463287830 |
| C | 7.173065662 | 1.743540168 | 9.829255104 |
| C | 3.658184290 | 2.954509735 | 4.182983875 |
| C | 3.371579170 | 6.441590309 | 7.109559536 |
| C | 6.178966999 | 7.543470860 | 10.314157486 |
| C | 0.850796580 | 1.852629185 | 0.978385985 |
| C | 4.365678310 | 2.845420837 | 6.624657631 |
| C | 2.664085627 | 6.550679207 | 4.667885780 |
| C | 6.138798714 | 6.047799587 | 10.156174660 |
| C | 0.890964866 | 3.348300219 | 1.136368632 |
| C | 4.405846119 | 1.349750280 | 6.782639980 |
| C | 2.623916864 | 8.046350479 | 4.509903431 |
| C | 6.043296337 | 0.195250645 | 3.097770691 |
| C | 0.986466765 | 9.200849533 | 8.194772720 |
| C | 6.233385086 | 4.893300533 | 2.548501015 |
| C | 0.796378434 | 4.502799511 | 8.744042397 |
| H | 6.011835575 | 9.003342628 | 0.397497535 |
| H | 1.017927766 | 0.392757177 | 10.895046234 |
| H | 6.264846325 | 4.305292606 | 5.248774052 |
| H | 0.764917433 | 5.090807438 | 6.043769360 |
| H | -0.290265769 | 8.162392616 | 3.463423014 |
| H | 7.320029259 | 1.233707666 | 7.829120636 |
| H | 3.805147648 | 3.464342356 | 2.182848692 |
| H | 3.224615812 | 5.931757927 | 9.109694481 |
| H | 0.671045184 | 7.147613049 | 1.400275350 |
| H | 6.358718395 | 2.248486757 | 9.892268181 |
| H | 2.843836546 | 2.449563265 | 4.245995998 |
| H | 4.185926437 | 6.946537018 | 7.046547413 |
| H | 7.008801937 | 7.879569530 | 9.966798782 |
| H | 0.020961139 | 1.516530752 | 1.325744629 |
| H | 3.535842896 | 3.181518793 | 6.972016335 |
| H | 3.493920803 | 6.214580536 | 4.320527077 |
| H | 5.465198040 | 7.928429127 | 9.799669266 |
| H | 1.564565182 | 1.467670798 | 1.492874265 |
| H | 5.079446793 | 3.230379820 | 7.139145851 |
| H | 1.950316429 | 6.165720940 | 4.153397560 |
| H | 6.902689934 | 5.665848255 | 10.595793724 |
| H | 0.127073571 | 3.730251789 | 0.696749926 |
| H | 3.641955137 | 0.967797577 | 6.343021393 |
| H | 3.387808084 | 8.428301811 | 4.949522018 |

| | | | |
|---|---|---|---|
| H | 6.158972740 | 5.819005013 | 9.223749161 |
| H | 0.870790660 | 3.577095270 | 2.068794012 |
| H | 4.385672569 | 1.120954752 | 7.715065479 |
| H | 2.644090891 | 8.275145531 | 3.577477694 |
| H | 5.335652351 | 5.702492714 | 10.552881241 |
| H | 1.694111109 | 3.693607092 | 0.739661574 |
| H | 5.208992958 | 1.004442930 | 6.385933399 |
| H | 1.820770502 | 8.391656876 | 4.906610012 |
| H | 6.498447895 | 0.981893003 | 3.405831099 |
| H | 0.531315327 | 8.414207458 | 7.886712551 |
| H | 5.778233528 | 5.679943085 | 2.240440607 |
| H | 1.251530290 | 3.716156960 | 9.052103043 |
| H | 5.810043335 | 9.040926933 | 3.849628210 |
| H | 1.219720006 | 0.355172724 | 7.442915440 |
| H | 6.466638088 | 4.342876911 | 1.796643615 |
| H | 0.563125193 | 5.053222656 | 9.495900154 |
| H | 5.245687485 | 0.450072825 | 2.627774954 |
| H | 1.784075975 | 8.946026802 | 8.664768219 |
| H | 7.030993938 | 5.148122787 | 3.018496990 |
| H | -0.001230230 | 4.247977257 | 8.274046898 |
